# Supplementary material for: Privacy-Preserving, Communication-Efficient, and Target-Flexible Hospital Quality Measurement
Source: arXiv:2203.00768 source file (2023-02-06)
Supplement: Supplementary file 2 [file supplement.pdf]

# Supplementary Materials for Privacy-Preserving, Communication-Efficient, and Target-Flexible Hospital Quality Measurement

Larry Han<sup>\*</sup>   Yige Li<sup>†</sup>   Bijan A. Niknam<sup>‡</sup>   José R. Zubizarreta<sup>§</sup>

## Overview of Supplementary Materials

The supplement consists of four appendices. In Appendix I, we prove the data-adaptive property of the hospital-level weights. In Appendix II, we show how patient-level information is not required to solve for the data-adaptive hospital-level weights (i.e., summary-level information is sufficient). Appendix III and Appendix IV contain additional results from the simulation study and real data analysis, respectively.

---

<sup>\*</sup>Department of Biostatistics, Harvard T.H. Chan School of Public Health; [larryhan@g.harvard.edu](mailto:larryhan@g.harvard.edu).

<sup>†</sup>Department of Biostatistics and CAUSALab, Harvard T.H. Chan School of Public Health.

<sup>‡</sup>Department of Health Care Policy and CAUSALab, Harvard University.

<sup>§</sup>Departments of Health Care Policy, Biostatistics, and Statistics, and CAUSALab, Harvard University.

# Appendix I. Derivation of Influence Functions

## General Form of Influence Functions

In this section, we summarize the general form of the influence functions for the target and source site estimators. The influence function in the target site  $\xi_{i,T}^{(a)}$  is

$$\sqrt{N}(\hat{\mu}_T^{(a)} - \mu_T^{(a)}) = \frac{1}{\sqrt{N}} \sum_{i=1}^N \frac{I(R_i = T)}{\rho_T} \xi_{i,T}^{(a)} + o_p(1),$$

where

$$\begin{aligned} \xi_{i,T}^{(a)} = & \frac{I(A_i = a)Y_i}{\pi_a(\mathbf{X}_i; \boldsymbol{\alpha}^*)} - \left( \frac{I(A_i = a)}{\pi_a(\mathbf{X}_i; \boldsymbol{\alpha}^*)} - 1 \right) m_a(\mathbf{X}_i; \boldsymbol{\beta}_a^*) - \mu_T^{(a)} \\ & + D_1(\boldsymbol{\alpha}^*, \boldsymbol{\beta}_a^*) \phi_T(\mathbf{X}_i; \boldsymbol{\alpha}^*) + D_2(\boldsymbol{\alpha}^*, \boldsymbol{\beta}_a^*) I_T \nabla f(\mathbf{X}_i, Y_i, \boldsymbol{\beta}_a^*), \end{aligned}$$

where  $D_1(\boldsymbol{\alpha}^*, \boldsymbol{\beta}_a^*) = \mathbb{E}[(Y_i - m_a(\mathbf{X}_i; \boldsymbol{\beta}_a^*))(-\mathbf{X}_i^\top \exp(\boldsymbol{\alpha}^{*\top} \mathbf{X}_i) I(A_i = a))]$ ,

$$D_2(\boldsymbol{\alpha}^*, \boldsymbol{\beta}_a^*) = \mathbb{E} \left[ \mathbf{X}_i^\top \left\{ \frac{I(A_i = a)}{\pi_a(\mathbf{X}_i; \boldsymbol{\alpha}^*)} - 1 \right\} \right],$$

$$I_T = \mathbb{E} [\nabla^2 L_T]^{-1} = \mathbb{E} \left[ \nabla^2 \left[ \frac{1}{N_T} \sum_{i=1}^{N_T} (Y_i - \boldsymbol{\beta}_a^{*\top} \mathbf{X}_i)^2 \right] \right]^{-1} = \mathbb{E} \left[ \frac{2}{N_T} \sum_{i=1}^{n_i} (\mathbf{X}_i^\top \mathbf{X}_i) \right]^{-1},$$

$$\phi_T(\mathbf{X}_i; \boldsymbol{\alpha}^*) = \mathbb{E} [\mathbf{X}_i^\top \pi_a(\mathbf{X}_i; \boldsymbol{\alpha}^*) (1 - \pi_a(\mathbf{X}_i; \boldsymbol{\alpha}^*) \mathbf{X}_i)^{-1} \{ \mathbf{X}_i^\top (I(A_i = a) - \pi_a(\mathbf{X}_i; \boldsymbol{\alpha}^*)) \}],$$

and  $\nabla f(\mathbf{X}_i, Y_i, \boldsymbol{\beta}_a^*) = -2\mathbf{X}_i^\top (Y_i - \boldsymbol{\beta}_a^{*\top} \mathbf{X}_i)$  for a linear outcome  $Y_i$ . When the outcome regression model is correctly specified,  $D_1(\boldsymbol{\alpha}^*, \boldsymbol{\beta}_a^*) = 0$ , and when the propensity score model is correctly specified,  $D_2(\boldsymbol{\alpha}^*, \boldsymbol{\beta}_a^*) = 0$ .

In the source sites, we must additionally consider estimation of the density ratio weights.

Let  $h(\mathbf{X}_i; \boldsymbol{\gamma}_k, \tau) = \mathbf{X}_i \exp(\boldsymbol{\gamma}_k^\top \mathbf{X}_i) - \tau$ , where  $\mathbf{X} = (1, X_1, \dots, X_p)^\top$  is a design matrix with 1 in the first column and  $\tau = (1, E_1(\mathbf{X}))^\top$  is the covariate mean vector in the target population

with 1 in the first entry. By a Taylor series expansion, we can obtain that

$$\begin{aligned}\sqrt{N}(\hat{\gamma}_k - \gamma_k^*) &= \frac{1}{\sqrt{N}\rho_k} \sum_{i=1}^N \left\{ H_1^{-1} h(\mathbf{X}_i; \gamma_k^*, \tau^*) I(R_i = k) \right. \\ &\quad \left. + \sqrt{\frac{\rho_k}{\rho_T}} H_1^{-1} (\mathbf{X}_i - \tau) I(R_i = T) \right\} + o_p(1),\end{aligned}$$

where  $H_1 = \mathbb{E}[-\mathbf{X}_i \exp(\gamma_k^{*\top} \mathbf{X}_i) \mathbf{X}_i^\top]$ .

Then the source site influence function is

$$\begin{aligned}\sqrt{N}(\hat{\mu}_k^{(a)} - \mu_k^{(a)}) &= \frac{1}{\sqrt{N}\rho_k} \sum_{i=1}^N \left\{ I(R_i = T) m_a(\mathbf{X}_i; \beta_a^*) - \mu_k^{(a)} \right. \\ &\quad + [Y_i - m_a(\mathbf{X}_i; \beta_a^*)] \left[ \frac{I(R_i = k, A_i = a) \omega_k(\mathbf{X}_i; \gamma_k^*)}{\pi_{a,k}(\mathbf{X}_i; \alpha_k^*)} + 2D_2^k(\alpha_k^*, \beta_a^*) I_k \mathbf{X}_i \right] \\ &\quad \left. + D_1^k(\alpha_k^*) IF_i(\mathbf{X}_i; \alpha_k^*) + D_1^k(\gamma_k^*) IF_i(\mathbf{X}_i; \gamma_k^*) \right\} + o_p(1),\end{aligned}$$

where  $D_2^k(\alpha_k^*, \beta_a^*) = \mathbb{E} \left[ \mathbf{X}_i^T \left( \frac{I(R_i = k, A_i = a) \omega_k(\mathbf{X}_i; \gamma_k^*)}{\pi_{a,k}(\mathbf{X}_i; \alpha_k^*)} - 1 \right) \right]$ ,

$I_k = [\mathbb{E} \nabla^2 L_k(\beta_a^*)]^{-1} = \left[ \mathbb{E} \left( \frac{2}{n_k} \sum_{i=1}^{n_k} \mathbf{X}_i^T \mathbf{X}_i \right) \right]^{-1}$ ,

$D_{1, \alpha_k^*}^k = \mathbb{E} \left[ \{Y_i - m_a(\mathbf{X}_i; \beta_a^*)\} I(R_i = k, A_i = a) \exp(\gamma_k^{*\top} \mathbf{X}_i) \mathbf{X}_i \frac{\pi_{a,k}(\mathbf{X}_i; \alpha_k^*) - 1}{\pi_{a,k}(\mathbf{X}_i; \alpha_k^*)} \right]$ ,

$IF_i(\mathbf{X}_i; \alpha_k^*) = [\mathbb{E}(\mathbf{X}_i^\top \pi_{a,k}(\mathbf{X}_i; \alpha_k^*) (1 - \pi_{a,k}(\mathbf{X}_i; \alpha_k^*)) \mathbf{X}_i)]^{-1} \mathbf{X}_i \cdot (I(A_i = a) - \pi_{a,k}(\mathbf{X}_i; \alpha_k^*))$ ,

$D_{1, \gamma_k^*}^k = \mathbb{E} \left[ \{Y_i - m_a(\mathbf{X}_i; \beta_a^*)\} I(R_i = k, A_i = a) \mathbf{X}_i \exp(\gamma_k^{*\top} \mathbf{X}_i) \frac{\exp(\alpha_k^{*\top} \mathbf{X}_i)}{1 + \exp(\alpha_k^{*\top} \mathbf{X}_i)} \right]$ ,

$IF_i(\mathbf{X}_i; \gamma_k^*) = H_1^{-1} h(\mathbf{X}_i; \gamma_k^*, \tau^*) I(R_i = k) + \sqrt{\frac{n_k}{N_T}} H_1^{-1} I(R_i = T) (\mathbf{X}_i - \tau)$ .

## Derivation of the Target Influence Function

Suppose we have an estimator from the target site,  $\hat{\mu}_{a,T}^T$  of the true  $\mu_{a,T}$  for  $a = 0, 1$ . Suppose that the sample size in the target site is  $N_T$ . In the propensity score model, suppose that

$\widehat{\boldsymbol{\alpha}} - \boldsymbol{\alpha}^* = o_p(1)$ . In the outcome regression model, suppose also that  $\widehat{\boldsymbol{\beta}}_a - \boldsymbol{\beta}_a^* = o_p(1)$ . Then the influence function for  $\widehat{\mu}_{a,T}$  can be decomposed as

$$\begin{aligned}
\sqrt{N_T} (\widehat{\mu}_{a,T}^T - \mu_{a,T}) &= \frac{1}{\sqrt{N_T}} \sum_{i=1}^{N_T} \left[ \frac{I(A_i = a)Y_i}{\pi_a(X_i, \widehat{\boldsymbol{\alpha}})} - \left( \frac{I(A_i = a)}{\pi_a(X_i, \widehat{\boldsymbol{\alpha}})} - 1 \right) m_a(X_i, \widehat{\boldsymbol{\beta}}_a) - \mu_{a,T} \right] \\
&= \underbrace{\frac{1}{\sqrt{N_T}} \sum_{i=1}^{N_T} \left[ \frac{I(A_i = a)Y_i}{\pi_a(X_i, \boldsymbol{\alpha}_k^*)} - \left( \frac{I(A_i = a)}{\pi_a(X_i, \boldsymbol{\alpha}_k^*)} - 1 \right) m_a(X_i, \boldsymbol{\beta}_a^*) - \mu_{a,T} \right]}_{T_1} \\
&\quad + \underbrace{\frac{1}{\sqrt{N_T}} \sum_{i=1}^{N_T} \left[ I(A_i = a) \left( \frac{1}{\pi_a(X_i, \widehat{\boldsymbol{\alpha}})} - \frac{1}{\pi_a(X_i, \boldsymbol{\alpha}_k^*)} \right) \{Y_i - m_a(X_i, \boldsymbol{\beta}_a^*)\} \right]}_{T_2} \\
&\quad - \underbrace{\frac{1}{\sqrt{N_T}} \sum_{i=1}^{N_T} \left[ \left\{ \frac{I(A_i = a)}{\pi_a(X_i, \boldsymbol{\alpha}_k^*)} - 1 \right\} \{m_a(X_i, \widehat{\boldsymbol{\beta}}_a) - m_a(X_i, \boldsymbol{\beta}_a^*)\} \right]}_{T_3} \\
&\quad - \underbrace{\frac{1}{\sqrt{N_T}} \sum_{i=1}^{N_T} \left[ I(A_i = a) \left( \frac{1}{\pi_a(X_i, \widehat{\boldsymbol{\alpha}})} - \frac{1}{\pi_a(X_i, \boldsymbol{\alpha}_k^*)} \right) \{m_a(X_i, \widehat{\boldsymbol{\beta}}_a) - m_a(X_i, \boldsymbol{\beta}_a^*)\} \right]}_{T_4}
\end{aligned}$$

If either the outcome regression model or propensity score model is correctly specified, then  $\mathbb{E}(T_1) = 0$ . For  $T_2$ , when the outcome regression model is correctly specified but the propensity score model may be misspecified,  $T_2 = o_p(1)$ . To show this, note that since  $\widehat{\boldsymbol{\alpha}} \rightarrow \boldsymbol{\alpha}^*$ , then  $\frac{1}{\pi_a(X_i, \widehat{\boldsymbol{\alpha}})} - \frac{1}{\pi_a(X_i, \boldsymbol{\alpha}^*)} = o_p(1)$ . Let  $D_i = I(A_i = a) \left( \frac{1}{\pi_a(X_i, \widehat{\boldsymbol{\alpha}})} - \frac{1}{\pi_a(X_i, \boldsymbol{\alpha}^*)} \right) \{Y_i - m_a(X_i, \boldsymbol{\beta}_a^*)\}$ . Given  $X_i$ ,  $i = 1, \dots, N_T$ ,  $D_i \perp D_j$  for  $i \neq j$  and  $\mathbb{E}(D_i | X_i) = 0$ . Since  $\text{Var}(D_i | X_i) \leq \max(\pi_i(\boldsymbol{\alpha}^*) - \pi_i(\widehat{\boldsymbol{\alpha}}))^2 \rightarrow o_p(1)$ , then for any  $\epsilon > 0$ , by Chebyshev's inequality,

$$P_{D|X} \left( \left| N_T^{-1/2} \sum_{i=1}^{N_T} D_i \right| \geq \epsilon \right) \leq \frac{\text{Var}(D_i | X_i)}{\epsilon^2} \leq o_p(1),$$

so  $T_2 = o_p(1)$ . But when the outcome regression model is misspecified, then  $\mathbb{E}[Y - m_a(X, \boldsymbol{\beta}_a^*)] \neq 0$ , and the uncertainty of  $\widehat{\boldsymbol{\alpha}}$  contributes to the uncertainty of  $\widehat{\mu}_{a,T}^T$ , i.e.,

we need to consider the uncertainty contribution from the estimation of  $\widehat{\alpha}$ . By a similar argument,  $T_3 = o_p(1)$  when the propensity score model is correctly specified. However, when it is misspecified, the influence function of  $\widehat{\beta}_a$  must be considered as it will contribute to the influence function of  $\widehat{\mu}_{a,T}^T$ . For  $T_4$  to be  $o_p(1)$ , it suffices that the product

$$\{\pi_a(X_i, \widehat{\alpha})^{-1} - \pi_a(X_i, \alpha^*)^{-1}\} \cdot \{m_a(X_i, \widehat{\beta}_a) - m_a(X_i, \beta_a^*)\}$$

be  $O_p(n^{-d})$  where  $d > 1/2$ , which is easily satisfied if  $\alpha$  and  $\beta_a$  are estimated by maximum likelihood, in which case the product converges at rate  $O_p(n^{-1})$ . In the general case where models may be misspecified, we need to plug-in the influence functions for  $\widehat{\alpha} - \alpha^*$  and  $\widehat{\beta}_a - \beta_a^*$ .

Denote

$$g_0(X_i, \alpha) := \frac{I(A_i = a)}{\pi_a(X_i, \alpha)},$$

so that we can write  $T_2$  as

$$\begin{aligned} T_2 &= N_T^{-1/2} \sum_{i=1}^{N_T} [Y_i - m_a(X_i, \beta_a^*)] [g_0(X_i, \widehat{\alpha}) - g_0(X_i, \alpha^*)] \\ &= N_T^{-1/2} \sum_{i=1}^{N_T} [Y_i - m_a(X_i, \beta_a^*)] \nabla g_0(X_i, \alpha') (\widehat{\alpha} - \alpha^*) \\ &= N_T^{-1/2} \sum_{i=1}^{N_T} [Y_i - m_a(X_i, \beta_a^*)] \nabla g_0(X_i, \alpha^*) (\widehat{\alpha} - \alpha^*) \\ &\quad + N_T^{-1/2} \sum_{i=1}^{N_T} [Y_i - m_a(X_i, \beta_a^*)] \underbrace{[\nabla g_0(X_i, \alpha') - \nabla g_0(X_i, \alpha^*)]}_{o_p(\sqrt{N_T})} (\widehat{\alpha} - \alpha^*) \\ &\quad \underbrace{\hspace{10em}}_{o_p(1)} \\ &= N_T^{-1} \sum_{i=1}^{N_T} [Y_i - m_a(X_i, \beta_a^*)] \nabla g_0(X_i, \alpha^*) \cdot \sqrt{N_T} (\widehat{\alpha} - \alpha^*) + o_p(1), \end{aligned}$$

where  $\|\alpha' - \alpha^*\| < \|\widehat{\alpha} - \alpha^*\|$ .

By the law of large numbers,

$$N_T^{-1} \sum_{i=1}^{N_T} [Y_i - m_a(X_i, \beta_a^*)] \nabla g_0(X_i, \alpha^*) \rightarrow \mathbb{E} [[Y_i - m_a(X_i, \beta_a^*)] \nabla g_0(X_i, \alpha^*)] = D_1(\beta_a^*, \alpha^*).$$

Further assume that  $\sqrt{N_T}(\widehat{\alpha} - \alpha^*) = N_T^{-1/2} \sum_{i=1}^{N_T} \phi_T(\mathbf{X}_i; \alpha)$  where  $\phi_T(\mathbf{X}_i; \alpha)$  is the influence function for  $\widehat{\alpha}$ . Then

$$T_2 = N_T^{-1/2} \sum_{i=1}^{N_T} D_1(\beta_a^*, \alpha^*) \cdot \phi_T(\mathbf{X}_i; \alpha) + o_p(1).$$

If the outcome regression model is correctly specified, then

$$D_1 = \mathbb{E}_{X,A} \{ \nabla g_0(X_i, \alpha^*) \mathbb{E}_{Y|X,A} [Y_i - m_a(X_i, \beta_a^*)] \} = 0,$$

and  $T_2 = o_p(1)$ .

Now focusing on  $T_3$ , we can write

$$\begin{aligned} T_3 &= \frac{1}{\sqrt{N_T}} \sum_{i=1}^{N_T} \left[ \left\{ \frac{I(A_i = a)}{\pi_a(X_i, \alpha^*)} - 1 \right\} \{m_a(X_i, \widehat{\beta}_a) - m_a(X_i, \beta_a^*)\} \right] \\ &= \frac{1}{\sqrt{N_T}} \sum_{i=1}^{N_T} \left[ \left\{ \frac{I(A_i = a)}{\pi_a(X_i, \alpha^*)} - 1 \right\} \nabla m_a(X_i, \beta_a^*)(\widehat{\beta}_a - \beta_a^*) \right] + o_p(1) \\ &= N_T^{-1} \sum_{i=1}^{N_T} \left[ \left\{ \frac{I(A_i = a)}{\pi_a(X_i, \alpha^*)} - 1 \right\} \nabla m_a(X_i, \beta_a^*) \right] \cdot \sqrt{N_T}(\widehat{\beta}_a - \beta_a^*) + o_p(1). \end{aligned}$$

By the law of large numbers,

$$N_T^{-1} \sum_{i=1}^{N_T} \left[ \left\{ \frac{I(A_i = a)}{\pi_a(X_i, \alpha^*)} - 1 \right\} \nabla m_a(X_i, \beta_a^*) \right] \rightarrow \mathbb{E} \left[ \left\{ \frac{I(A_i = a)}{\pi_a(X_i, \alpha^*)} - 1 \right\} \nabla m_a(X_i, \beta_a^*) \right] = D_2(\alpha^*, \beta_a^*).$$

How do we estimate  $\beta_a$ ? Suppose  $\beta_a$  is estimated within each site so that

$$\widehat{\beta}_{ak} = \arg \min_{\beta_a} L_k(\beta_a) = \arg \min_{\beta_a} n_k^{-1} \sum_{i=1}^{n_k} f(X_i, Y_i, \beta_a),$$

for some specified loss function  $f$ . For example,  $f(x, y, \beta_a) = (y - \beta_a^\top x)^2$  for linear regression, and  $f(x, y, \beta_a) = \log\{1 + \exp(\beta_a^\top x)\} - y\beta_a^\top x$  for logistic regression. By a Taylor series expansion of the gradient,

$$0 = \nabla L_k(\widehat{\beta}_{ak}) = \nabla L_k(\beta_a^*) + \nabla^2 L_k(\beta_a')(\widehat{\beta}_{ak} - \beta_a^*),$$

where  $\|\beta_a' - \beta_a^*\| \leq \|\widehat{\beta}_{ak} - \beta_a^*\|$ . This implies that

$$\sqrt{n_k} \mathbb{E} \nabla^2 L_k(\beta_a^*)(\widehat{\beta}_{ak} - \beta_a^*) = \sqrt{n_k} \nabla L_k(\beta_a^*) + \underbrace{\sqrt{n_k} (\nabla^2 L_k(\beta_a') - \mathbb{E} \nabla^2 L_k(\beta_a^*))(\widehat{\beta}_{ak} - \beta_a^*)}_{o_p(1)},$$

$$\text{since } \nabla^2 L_k(\beta_a') - \mathbb{E} \nabla^2 L_k(\beta_a^*) = \underbrace{\nabla^2 L_k(\beta_a') - \nabla^2 L_k(\beta_a^*)}_{\text{by Lipschitz } C\|\beta_{ak} - \beta_a^*\| \rightarrow O_p(n^{-1/2})} + \underbrace{\nabla^2 L_k(\beta_a^*) - \mathbb{E} \nabla^2 L_k(\beta_a^*)}_{\text{by Concentration } O_p(n^{-1/2})}.$$

Thus,

$$\sqrt{n_k}(\widehat{\beta}_{ak} - \beta_a^*) = \sqrt{n_k} \{\mathbb{E} \nabla^2 L_k(\beta_a^*)\}^{-1} \nabla L_k(\beta_a^*) + o_p(1).$$

Denoting  $\{E \nabla^2 L_k(\beta_a^*)\}^{-1}$  as  $I_k$ , we have

$$\sqrt{n_k}(\widehat{\beta}_{ak} - \beta_a^*) = n_k^{-1/2} \sum_{i=1}^{n_k} I_k \cdot \nabla f(x_i, y_i, \beta_a) + o_p(1).$$

If  $\widehat{\beta}_a = \widehat{\beta}_{0a}$ , using the outcome regression parameter fit in the target site, then

$$\sqrt{N_T}(\widehat{\beta}_{0a} - \beta_a^*) = N_T^{-1/2} \sum_{i=1}^{N_T} I_T \cdot \nabla f(x_i, y_i, \beta_a) + o_p(1).$$

Hence, we have

$$T_3 = N_T^{-1/2} \sum_{i=1}^{N_T} D_2 \cdot I_T \cdot \nabla f(x_i, y_i, \boldsymbol{\beta}_a) + o_p(1).$$

If the propensity score model is correctly specified, then

$$D_2 = \mathbb{E} \left[ \left( \frac{I(A_i = a)}{\pi(X_i, \boldsymbol{\alpha}^*)} - 1 \right) \nabla m_a(X_i, \boldsymbol{\beta}_a^*) \right] = 0,$$

and  $T_3 = o_p(1)$ .

Summarizing, since  $T_4 = o_p(1)$ , then combining  $T_1$ ,  $T_2$ , and  $T_3$ , we obtain the influence function in the target site to be

$$\begin{aligned} & \sqrt{N_T}(\hat{\mu}_{a,T}^T - \mu_{a,T}) \\ &= \frac{1}{\sqrt{N_T}} \sum_{i=1}^{N_T} \left\{ \frac{I(A_i = a)Y_i}{\pi_a(X_i, \boldsymbol{\alpha}^*)} - \left( \frac{I(A_i = a)}{\pi_a(X_i, \boldsymbol{\alpha}^*)} - 1 \right) m_a(X_i, \boldsymbol{\beta}_a^*) - \mu_{a,T} \right. \\ & \quad \left. + D_1 \phi_T(x_i, \alpha) + D_2 I_T \nabla f(X_i, Y_i, \boldsymbol{\beta}_a^*) \right\} + o_p(1) \end{aligned}$$

When both outcome regression and propensity score models are correct,  $D_1 = D_2 = 0$ , so the influence function reduces to

$$\begin{aligned} & \sqrt{N}(\hat{\mu}_{a,T}^T - \mu_{a,T}) \\ &= \frac{1}{\sqrt{N}\rho_T} \sum_{i=1}^N I(R_i = T) \left\{ \frac{I(A_i = a)Y_i}{\pi_a(X_i, \boldsymbol{\alpha}^*)} - \left( \frac{I(A_i = a)}{\pi_a(X_i, \boldsymbol{\alpha}^*)} - 1 \right) m_a(X_i, \boldsymbol{\beta}_a^*) - \mu_{a,T} \right\} + o_p(1). \end{aligned}$$

When the outcome regression model is correct, but the propensity score model may be



misspecified,  $D_1 = 0$ , so the influence function reduces to

$$\begin{aligned} & \sqrt{N}(\widehat{\mu}_{a,T}^T - \mu_{a,T}) \\ &= \frac{1}{\sqrt{N}\rho_T} \sum_{i=1}^N I(R_i = T) \left\{ \{Y_i - m_a(X_i, \beta_a^*)\} \left[ \frac{I(A_i = a)}{\pi_a(X_i, \alpha^*)} + 2D_2 I_T X_i \right] + m_a(X_i, \beta_a^*) - \mu_{a,T} \right\} + o_p(1), \end{aligned}$$

since  $\nabla f(X_i, Y_i, \beta_a^*) = 2X_i^\top (Y_i - m_a(X_i, \beta_a^*))$ .

When the propensity score model is correct, but the outcome regression model may be misspecified,  $D_2 = 0$ , so the influence function reduces to

$$\begin{aligned} & \sqrt{N_T}(\widehat{\mu}_{a,T}^T - \mu_{a,T}) \\ &= \frac{1}{\sqrt{N_T}} \sum_{i=1}^{N_T} \left\{ \frac{I(A_i = a)Y_i}{\pi_a(X_i, \alpha^*)} - \left( \frac{I(A_i = a)}{\pi_a(X_i, \alpha^*)} - 1 \right) m_a(X_i, \beta_a^*) - \mu_{a,T} + D_1 \phi_T(x_i, \alpha) \right\} + o_p(1). \end{aligned}$$

It remains to obtain  $\phi_T(x_i, \alpha)$ . We follow the general strategy to find  $\widehat{\alpha}$  that solves the system of moment equations,  $E[h(X_i, \alpha)] = 0$ . Since the system is exactly identified, the variance can be estimated as  $\widehat{Var}(\widehat{\alpha}) = n^{-1}B^{-1}(\widehat{\alpha})M(\widehat{\alpha})B^{-1}(\widehat{\alpha})^\top$ , where  $B(\widehat{\alpha}) = -n^{-1} \sum_{i=1}^n \frac{\partial h(X_i, \alpha)}{\partial \alpha^\top} \big|_{\alpha=\widehat{\alpha}}$  and  $M(\widehat{\alpha}) = n^{-1} \sum_{i=1}^n h(X_i, \widehat{\alpha})h(X_i, \widehat{\alpha})^\top$ . Based on M-estimation theory and the theory of influence functions,  $\widehat{Var}(\widehat{\alpha}) = n^{-1}(n^{-1} \sum_{i=1}^n IF_i(\widehat{\alpha})IF_i(\widehat{\alpha})^\top)$ . It is clear that

$$IF_i(\alpha) = \mathbb{E}[B(\alpha)]^{-1} h(X_i, \alpha).$$

For  $\phi_T(x_i, \alpha)$  where the propensity score is estimated by logistic regression,  $P(A_i = 1 \mid X_i) = \pi_a(X_i, \alpha) = \frac{\exp(\alpha^\top x)}{1 + \exp(\alpha^\top x)}$ . Then  $h(X_i, \alpha) = X_i^\top (A_i - \pi_a(X_i, \alpha))$  and  $\frac{\partial h(X_i, \alpha)}{\partial \alpha^\top} = -X_i^\top [\pi_a(X_i, \alpha)(1 - \pi_a(X_i, \alpha))] X_i$ . Hence

$$\phi_T(X_i, \alpha) = E[X_i^\top \pi_a(X_i, \alpha)(1 - \pi_a(X_i, \alpha))X_i]^{-1} \cdot X_i^\top (I(A_i = a) - \pi_a(X_i, \alpha)).$$

The influence function  $\sqrt{N}(\widehat{\mu}_{a,T}^T - \mu_{a,T})$  reduces to

$$\begin{aligned} \sqrt{N}(\widehat{\mu}_{a,T}^T - \mu_{a,T}) &= \frac{1}{\sqrt{N}\rho_T} \sum_{i=1}^N I(R_i = T) \left\{ \underbrace{\left( \frac{I(A_i = a)Y_i}{\pi_a(X_i, \boldsymbol{\alpha}^*)} - \mu_{a,T} \right)}_{\text{Mean 0}} \right. \\ &\quad \left. - \underbrace{\left( \frac{I(A_i = a)}{\pi_a(X_i, \boldsymbol{\alpha}^*)} - 1 \right) \cdot \left[ m_a(X_i, \boldsymbol{\beta}_a^*) + G_1 G_2^{-1} \pi_a(X_i, \boldsymbol{\alpha}^*) X_i^\top \right]}_{\text{Mean 0 under correct PS model}} \right\} + o_p(1), \end{aligned}$$

where

$$G_1 = \mathbb{E} \left[ [Y_i - m_a(X_i, \boldsymbol{\beta}_a^*)] I(A_i = a) \frac{X_i(\pi_a(X_i, \boldsymbol{\alpha}^*) - 1)}{\pi_a(X_i, \boldsymbol{\alpha}^*)} \right]$$

and

$$G_2 = \mathbb{E} [X_i^\top \pi_a(X_i, \boldsymbol{\alpha}^*) (1 - \pi_a(X_i, \boldsymbol{\alpha}^*)) X_i].$$

## Source Sites

In the source sites, we must additionally consider estimation of the density ratio weights.

Let  $h(X_i, \boldsymbol{\gamma}_k, \tau) = X_i \exp(\boldsymbol{\gamma}_k^\top X_i) - \tau$ , where  $X = (1, X_1, \dots, X_p)^\top$  is a design matrix with 1 in the first column and  $\tau = (1, E_T(X))^\top$  is the covariate mean vector in the target population with 1 in the first entry.

$$\begin{aligned} 0 &= n_k^{-1} \sum_{i=1}^{n_k} h(X_i, \widehat{\boldsymbol{\gamma}}_k, \widehat{\tau}) \\ &= \frac{1}{\sqrt{n_k}} \sum_{i=1}^{n_k} h(X_i, \boldsymbol{\gamma}_k^*, \tau^*) + n_k^{-1} \sum_{i=1}^{n_k} \nabla_{\boldsymbol{\gamma}_k} h(X_i, \boldsymbol{\gamma}_k', \tau') \cdot \sqrt{n_k}(\widehat{\boldsymbol{\gamma}}_k - \boldsymbol{\gamma}_k^*) \\ &\quad + n_k^{-1} \sum_{i=1}^{n_k} \nabla_{\tau} h(X_i, \boldsymbol{\gamma}_k', \tau') \cdot \sqrt{n_k}(\widehat{\tau} - \tau^*) + o_p(1) \\ &\rightarrow \frac{1}{\sqrt{n_k}} \sum_{i=1}^{n_k} h(X_i, \boldsymbol{\gamma}_k^*, \tau^*) + \mathbb{E} [\nabla_{\boldsymbol{\gamma}_k} h(X_i, \boldsymbol{\gamma}_k', \tau')] \cdot \sqrt{n_k}(\widehat{\boldsymbol{\gamma}}_k - \boldsymbol{\gamma}_k^*) \\ &\quad + \mathbb{E} [\nabla_{\tau} h(X_i, \boldsymbol{\gamma}_k', \tau')] \cdot \sqrt{n_k}(\widehat{\tau} - \tau^*) + o_p(1) \end{aligned}$$

Re-arranging for  $\sqrt{n_k}(\hat{\gamma}_k - \gamma_k^*)$ ,

$$\begin{aligned}\sqrt{n_k}(\hat{\gamma}_k - \gamma_k^*) &= \frac{1}{\sqrt{n_k}} \sum_{i=1}^{n_k} H_1^{-1} h(X_i, \gamma_k^*, \tau^*) + H_1^{-1} \sqrt{n_k}(\hat{\tau} - \tau^*) \\ &= \frac{1}{\sqrt{n_k}} \sum_{i=1}^{n_k} H_1^{-1} h(X_i, \gamma_k^*, \tau^*) + \sqrt{\frac{\rho_k}{\rho_T}} H_1^{-1} \sum_{i=1}^N [I(R_i \in T)(X_i - \tau)],\end{aligned}$$

where  $H_1 = \mathbb{E}[-\nabla_{\gamma_k} h(X_i, \gamma_k^*, \tau^*)]$ .

Then

$$\sqrt{N}(\hat{\gamma}_k - \gamma_k^*) = \frac{1}{\sqrt{N}\rho_k} \sum_{i=1}^N \left\{ H_1^{-1} h(X_i, \gamma_k^*, \tau^*) I(R_i = k) + \sqrt{\frac{\rho_k}{\rho_T}} H_1^{-1} (X_i - \tau) I(R_i \in T) \right\} + o_p(1),$$

where  $H_1 = \mathbb{E}[-X \exp(\gamma_k^{*\top} X) X^\top]$ .

To summarize, when the outcome regression model, propensity score model, and density ratio model are all correctly specified, then

$$\begin{aligned}\sqrt{N}(\hat{\mu}_{a,T}^r - \mu_{a,T}) &= \frac{1}{\sqrt{N}\rho_k} \sum_{i=1}^N \left\{ I(R_i = T) m_a(X_i, \beta_a^*) - \mu_{a,T} \right. \\ &\quad \left. + \frac{I(R_i = k, A_i = a) \omega_k(X_i, \gamma_k^*)}{\pi_a(X_i, \alpha^*)} [Y_i - m_a(X_i, \beta_a^*)] \right\} + o_p(1)\end{aligned}$$

When only the outcome regression model is correctly specified, then

$$\begin{aligned}\sqrt{N}(\hat{\mu}_{a,T}^r - \mu_{a,T}) &= \frac{1}{\sqrt{N}\rho_k} \sum_{i=1}^N \left\{ I(R_i = T) m_a(X_i, \beta_a^*) - \mu_{a,T} \right. \\ &\quad \left. + \{Y_i - m_a(X_i, \beta_a^*)\} \left[ \frac{I(R_i = k, A_i = a) \omega_k(X_i, \gamma_k^*)}{\pi_a(X_i, \alpha^*)} + 2D_2^r I_k X_i \right] \right\} + o_p(1),\end{aligned}$$

where  $D_2^r = \mathbb{E} \left[ \left( \frac{I(A_i=a, T_i=k) \omega_k(X_i, \gamma_k^*)}{\pi_a(X_i, \alpha^*)} - 1 \right) \nabla m_a(X_i, \beta_a^*) \right]$  and  $I_k = [\mathbb{E}(\nabla^2 L_k(\beta_a^*))]^{-1}$ .

When the propensity score model and density ratio model are correctly specified but the outcome regression model may be misspecified, then

$$\begin{aligned}
& \sqrt{N}(\hat{\mu}_{a,T}^r - \mu_{a,T}) \\
&= \frac{1}{\sqrt{N} \rho_k} \sum_{i=1}^N \left\{ I(R_i = T) m_a(X_i, \beta_a^*) - \mu_{a,T} + \frac{I(R_i = k, A_i = a) \omega_k(X_i, \gamma_k^*)}{\pi_a(X_i, \alpha^*)} [Y_i - m_a(X_i, \beta_a^*)] \right. \\
&\quad \left. + \underbrace{\mathbb{E} \left[ \{Y_i - m_a(X_i, \beta_a^*)\} I(R_i = k, A_i = a) \exp(\gamma_k^{*\top} X_i) \frac{\pi_a(X_i, \alpha^*) - 1}{\pi_a(X_i, \alpha^*)} \right]}_{D_{1, \alpha^*}^r} \right. \\
&\quad \cdot \underbrace{[\mathbb{E}(X_i^\top \pi_a(X_i, \alpha^*) (1 - \pi_a(X_i, \alpha^*)) X_i)]^{-1} X_i \cdot (I(A_i = a) - \pi_a(X_i, \alpha^*))}_{IF_i(X_i, \alpha^*)} \\
&\quad \left. + \underbrace{\mathbb{E} \left[ \{Y_i - m_a(X_i, \beta_a^*)\} I(R_i = k, A_i = a) X_i \exp(\gamma_k^{*\top} X_i) \frac{\exp(\alpha^{*\top} X_i)}{1 + \exp(\alpha^{*\top} X_i)} \right]}_{D_{1, \gamma_k^*}^r} \right. \\
&\quad \left. \cdot \underbrace{H_1^{-1} h(X_i, \gamma_k^*, \tau^*) I(R_i = k) + \sqrt{\frac{n_k}{N_T}} H_1^{-1} I(R_i = T) (X_i - \tau)}_{IF_i(X_i, \gamma_k^*)} \right\} + o_p(1).
\end{aligned}$$

## Appendix II. Data-Adaptive Weights

In this section, we prove that given a suitable choice for  $\lambda$ , then  $\hat{\eta}_k = \arg \min_{\eta_k} \hat{Q}_a(\eta)$  are adaptive weights such that  $\hat{\eta}_k - \eta_k^* = O_p(n_k^{-1/2})$  when  $\bar{\delta}_k = 0$  and  $P(\hat{\eta}_k = 0) \rightarrow 1$  when  $\bar{\delta}_k \neq 0$ . Recall that

$$\hat{Q}_a(\eta) = \sum_{i=1}^N \left[ \hat{\xi}_{i,T}^{(a)} - \sum_{k \in S} \eta_k (\hat{\xi}_{i,T}^{(a)} - \hat{\xi}_{i,k}^{(a)} - \hat{\delta}_k) \right]^2 + \lambda \sum_{k \in S} |\eta_k| \hat{\delta}_k^2, \quad (1)$$

First consider the case when  $\bar{\delta}_k = 0$ . Then the  $\hat{Q}_a(\eta)$  function reduces to the sum of the squared error term. By the Central Limit Theorem, the normalized and centered estimator converges in distribution to a mean 0 normal distribution with asymptotic variance  $\Sigma$  given

by

$$\Sigma = \mathbb{E} \left[ \widehat{\xi}_{i,T}^{(a)} - \sum_{k \in S} \eta_k (\widehat{\xi}_{i,T}^{(a)} - \widehat{\xi}_{i,k}^{(a)} - \widehat{\delta}_k) \right]^2.$$

Solving for the minimizer of this asymptotic variance gives  $\eta_k^*$ ,

$$\begin{aligned} 0 = \frac{\partial \Sigma}{\partial \eta_k} &= 2\eta_k \mathbb{E} [\xi_{i,T}^{(a)} - \xi_{i,k}^{(a)}]^2 + 2\mathbb{E} [\xi_{i,T}^{(a)} (\xi_{i,k}^{(a)} - \xi_{i,T}^{(a)})] \\ \implies \eta_k^* &= \frac{\mathbb{E} [\xi_{i,T}^{(a)2} - \xi_{i,T}^{(a)} \xi_{i,k}^{(a)}]}{\mathbb{E} [\xi_{i,k}^{(a)} - \xi_{i,T}^{(a)}]^2} \\ &= \frac{\mathbb{E} [\xi_{i,T}^{(a)2}]}{\mathbb{E} [\xi_{i,k}^{(a)} - \xi_{i,T}^{(a)}]^2} \end{aligned}$$

since  $\xi_{i,T}^{(a)}$  and  $\xi_{i,k}^{(a)}$  are independent and  $E[\xi_{i,T}^{(a)}] = 0$ .

Now consider the case when  $\bar{\delta}_k \neq 0$ . The asymptotic variance is given by

$$\mathbb{E} \left[ \xi_{i,T}^{(a)} - \sum_{k=1}^K \eta_k (\xi_{i,T}^{(a)} - \xi_{i,k}^{(a)} - \widehat{\delta}_k) \right]^2 + \lambda \sum_{k=1}^K |\eta_k| \widehat{\delta}_k^2.$$

For simplicity, consider the case where there are two sites in total, with one target site and one source site. Taking the derivative of the asymptotic variance with respect to  $\eta_k$ , we obtain

$$\begin{aligned} 0 &= 2\eta_k \mathbb{E} [\xi_{i,T}^{(a)} - \xi_{i,k}^{(a)} - \widehat{\delta}_k]^2 + 2\mathbb{E} [\xi_{i,T}^{(a)} (\xi_{i,T}^{(a)} - \xi_{i,k}^{(a)} - \widehat{\delta}_k)] \\ \implies \eta_k^* &= \frac{\mathbb{E} [\xi_{i,T}^{(a)2}] + 1/2\lambda\widehat{\delta}_k^2}{\mathbb{E} [\xi_{i,T}^{(a)} - \xi_{i,k}^{(a)} - \widehat{\delta}_k]^2}. \end{aligned}$$

Then this can be estimated by

$$\widehat{\eta}_k = \frac{\sum_{i=1}^n \widehat{\xi}_{i,T}^{(a)2} + \lambda \widehat{\delta}_k^2 / 2n_k}{\sum_{i=1}^n [\widehat{\xi}_{i,T}^{(a)} - \widehat{\xi}_{i,k}^{(a)}]^2 + n \widehat{\delta}_k^2},$$

where it can be seen that  $Pr(\widehat{\eta}_k = 0) \rightarrow 1$  as  $n_k \rightarrow \infty$  if  $\widehat{\delta}_k \neq 0$ .

## Appendix II. Privacy-preserving Penalized Regression

In this section, we show that in the federated setting, we can solve for the  $\eta_k$  that minimizes the  $Q_a(\boldsymbol{\eta})$  function without sharing patient-level information from the influence functions. Recall that  $\xi_{i,T}^{(a)}$  is the influence function for the target site and  $\xi_{i,k}^{(a)}$  is the influence function for source site  $k$  such that

$$\begin{aligned}\sqrt{N}(\widehat{\mu}_j^{(a)} - \mu_T^{(a)}) &= \frac{1}{\sqrt{N}} \sum_{i=1}^N \xi_{i,T}^{(a)} + o_p(1), \\ \sqrt{N}(\widehat{\mu}_k^{(a)} - \mu_k^{(a)}) &= \frac{1}{\sqrt{N}} \sum_{i=1}^N \xi_{i,k}^{(a)} + o_p(1),\end{aligned}$$

To estimate  $\eta_k$ , we minimized a weighted  $\ell_1$  penalty function,

$$\widehat{Q}_a(\boldsymbol{\eta}) = \sum_{i=1}^N \left[ \widehat{\xi}_{i,T}^{(a)} - \sum_{k \in S} \eta_k (\widehat{\xi}_{i,T}^{(a)} - \widehat{\xi}_{i,k}^{(a)} - \widehat{\delta}_k) \right]^2 + \lambda \sum_{k \in S} |\eta_k| \widehat{\delta}_k^2, \quad (2)$$

where  $\eta_k \geq 0$  and  $\sum_{k=1}^K \eta_k = 1$ ,  $\widehat{\delta}_k = \widehat{\mu}_k^{(a)} - \widehat{\mu}_T^{(a)}$  is the estimated bias from source site  $k$ , and  $\lambda$  is a tuning parameter.

To see that patient-level influence function information is not required, denote

$$\tilde{Y}_i = \widehat{\xi}_{i,T}^{(a)}, \quad \tilde{\mathbf{X}}_{i,k} = \widehat{\xi}_{i,T}^{(a)} - \widehat{\xi}_{i,k}^{(a)} - \widehat{\delta}_k.$$

Then the first term of (1) can be written as

$$\begin{aligned}
(\tilde{Y} - \tilde{\mathbf{X}}\eta_k)^\top (\tilde{Y} - \tilde{\mathbf{X}}\eta_k) &= \tilde{Y}^\top \tilde{Y} + \eta_k^\top \tilde{\mathbf{X}}^\top \tilde{\mathbf{X}} \eta_k - 2\eta_k^\top \tilde{\mathbf{X}}^\top \tilde{Y} \\
&= \underbrace{\sum_{k=1}^K \tilde{Y}_k^\top \tilde{Y}_k}_{S_{\tilde{Y}}} + \underbrace{\eta_k^\top \sum_{k=1}^K \tilde{\mathbf{X}}_k^\top \tilde{\mathbf{X}}_k \eta_k}_{S_{\tilde{\mathbf{X}}}} - 2\eta_k^\top \underbrace{\sum_{k=1}^K \tilde{\mathbf{X}}_k^\top \tilde{Y}_k}_{S_{\tilde{\mathbf{X}}Y}},
\end{aligned}$$

where  $S_{\tilde{Y}}$  is a scalar,  $S_{\tilde{\mathbf{X}}}$  is a  $p \times p$  matrix, and  $S_{\tilde{\mathbf{X}}Y}$  is a  $1 \times p$ -vector. Thus, it suffices to share only  $S_{\tilde{Y}}$ ,  $S_{\tilde{\mathbf{X}}}$ , and  $S_{\tilde{\mathbf{X}}Y}$  with the leading site.

## Appendix III. Additional Simulation Study Results

Recall that in the simulation study, we considered five settings with  $K \in \{10, 20, 50\}$  total hospitals, and five estimators for the first wave simulation: one estimator using data from the target hospital only (Target-Only), two estimators using all sites that weights each site proportionally to its sample size (SS (naive), SS), and two estimators that employ the federated algorithm with alternative solvers (global- $\ell_2$ , global- $\ell_1$ ). In the second wave simulation about direct standardization, we compare the federated algorithm with the fixed-effects regression, where fixed-effects regression refers to fitting a linear regression with  $\mathbb{E}[Y|A, X, R] = \sum_{k=1}^K \beta_{0k} I(k = R) + \sum_{k=1}^K \beta_{Ak} I(k = R)A + X\beta$ .

### Distribution of observations

In the dense data setting of the first wave simulation,  $\mathcal{D}_{\text{dense}}$ , for the target hospital  $k = 1$ , for  $p = 1, \dots, P$ , we let the location parameter  $\Xi_{1p} = 0.15 + 0.05 \frac{1-p}{P-1}$ , the scale parameter  $\Omega_{1p} = 1$ , and the skewness parameter  $A_{1p} = 0$ . For source hospitals  $k = 2, \dots, K$ , if the sample size is greater than or equal to the third quartile,  $n_k \geq \text{Q3}(\{n_k\}_{k=1}^K)$ , we set  $A_{kp} = 3 \times 2/P$ .

If the sample size is less than or equal to the first quartile,  $n_k \leq Q1(\{n_k\}_{k=1}^K)$ , we set  $A_{kp} = -1 \times 2/P$ . If the sample size is greater than the first quartile and less than the third quartile,  $n_k \in (Q1(\{n_k\}_{k=1}^K), Q3(\{n_k\}_{k=1}^K))$ , we set  $A_{kp} = 0$ , which are the same as the parameters of the target hospital. In the sparse data setting,  $\mathcal{D}_{\text{sparse}}$ , we keep the location parameter  $\Xi_{1p} = 0.15 + 0.05 \frac{1-p}{P-1}$ , the scale parameter  $\Omega_{1p} = 1$ . For the source hospitals, if the sample size is greater than or equal to the  $65 - K/10$  quantiles, or less than or equal to the  $35 + K/10$  quantiles, we set  $A_{kp} = 2$  for  $p = 1, 2$ , and  $A_{kp} = 0$  for the remaining source hospitals and the target hospital. For  $P = 10$ , besides the two continuous covariates coming from the  $P = 2$  settings, the rest covariates are generated from Bernoulli distributions with mean  $\theta_{kp} = 0.45 + 0.1 \frac{p-3}{7}$ , where  $p = 3, \dots, 10$ , for all the source hospitals and  $\theta_{kp} = 0.5$  for the target hospital. We plot the observations in target and source hospitals for the  $\mathcal{D}_{\text{dense}}$  and  $\mathcal{D}_{\text{sparse}}$  data generating mechanisms when  $K = 10$  and  $P = 2$ .

In the second wave simulation where direct standardization is considered, we focus on comparison between federated algorithm and fixed-effects regression. We consider two settings with the same covariate distribution, only differing in their true ATEs. In the first setting, the true ATEs are uniform in all the hospitals. While in the second setting, the true ATEs vary across the hospitals.



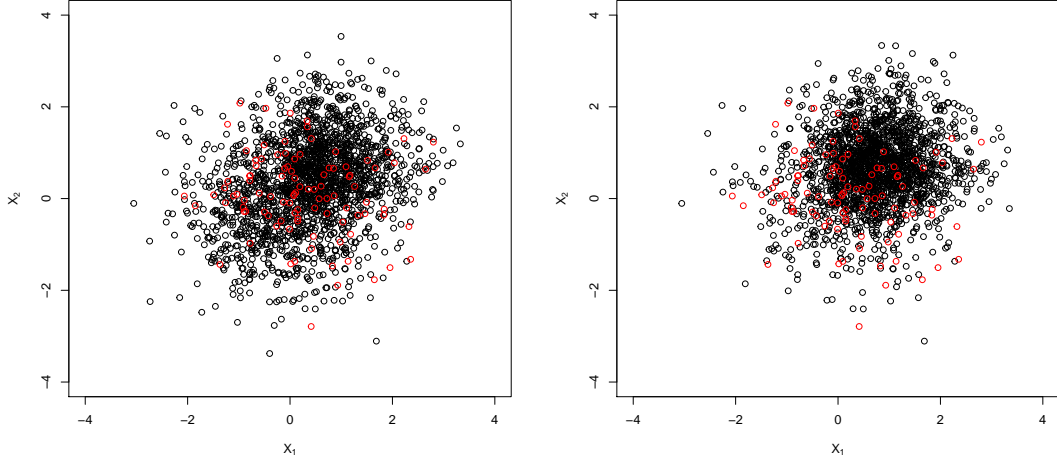

Figure 1: Red (black) dots are target (source) site observations ( $K = 10$ ,  $P = 2$ ). (Left) Dense covariate setting. (Right) Sparse covariate setting.

## Alternative number of covariates and distributions

In the main text, Table 1 reported simulation results for  $\mathcal{D}_{\text{sparse}}$  in Specifications I–V when  $P = 2$  covariates across 1000 simulations. Here, we present simulation results for  $\mathcal{D}_{\text{sparse}}$  when  $P = 10$  covariates and for  $\mathcal{D}_{\text{dense}}$  when  $P \in \{2, 10\}$ .

Table 1: See the main text.

Table 2: Results from 1000 simulated datasets for covariate distribution  $\mathcal{D}_{\text{sparse}}$  when  $P = 10$  with varying simulation settings and numbers of source sites.

|                   | Simulation scenarios |      |       |      |          |      |       |      |          |      |       |      |
|-------------------|----------------------|------|-------|------|----------|------|-------|------|----------|------|-------|------|
|                   | $K = 10$             |      |       |      | $K = 20$ |      |       |      | $K = 50$ |      |       |      |
|                   | Bias                 | RMSE | Cov.  | Len. | Bias     | RMSE | Cov.  | Len. | Bias     | RMSE | Cov.  | Len. |
| Specification I   |                      |      |       |      |          |      |       |      |          |      |       |      |
| Target-Only       | 0.01                 | 0.76 | 96.00 | 3.22 | 0.00     | 0.71 | 97.60 | 3.24 | 0.00     | 0.76 | 97.30 | 3.25 |
| SS (naive)        | 0.87                 | 0.88 | 27.20 | 1.46 | 0.90     | 0.91 | 2.40  | 0.87 | 0.92     | 0.92 | 0.00  | 0.46 |
| SS                | 0.10                 | 0.42 | 99.30 | 2.61 | 0.09     | 0.30 | 99.00 | 1.69 | 0.08     | 0.21 | 96.60 | 0.97 |
| GLOBAL $-\ell_2$  | 0.36                 | 0.51 | 96.40 | 2.26 | 0.41     | 0.52 | 87.00 | 1.56 | 0.44     | 0.50 | 54.00 | 0.90 |
| GLOBAL $-\ell_1$  | 0.16                 | 0.55 | 96.10 | 2.17 | 0.18     | 0.51 | 93.20 | 1.78 | 0.14     | 0.55 | 81.90 | 1.50 |
| Specification II  |                      |      |       |      |          |      |       |      |          |      |       |      |
| Target-Only       | 0.01                 | 0.82 | 95.90 | 3.32 | 0.01     | 0.74 | 97.40 | 3.31 | 0.00     | 0.79 | 97.20 | 3.33 |
| SS (naive)        | 0.87                 | 0.88 | 28.60 | 1.52 | 0.90     | 0.91 | 2.60  | 0.89 | 0.92     | 0.92 | 0.00  | 0.48 |
| SS                | 0.10                 | 0.42 | 99.30 | 2.68 | 0.09     | 0.31 | 99.30 | 1.71 | 0.08     | 0.21 | 97.00 | 0.99 |
| GLOBAL $-\ell_2$  | 0.37                 | 0.52 | 96.60 | 2.36 | 0.43     | 0.53 | 87.60 | 1.61 | 0.46     | 0.51 | 54.00 | 0.92 |
| GLOBAL $-\ell_1$  | 0.16                 | 0.57 | 95.00 | 2.25 | 0.19     | 0.52 | 93.50 | 1.80 | 0.13     | 0.59 | 80.60 | 1.56 |
| Specification III |                      |      |       |      |          |      |       |      |          |      |       |      |
| Target-Only       | 0.04                 | 0.76 | 95.60 | 3.24 | 0.06     | 0.74 | 96.40 | 3.24 | 0.06     | 0.79 | 96.70 | 3.29 |
| SS (naive)        | 0.84                 | 0.86 | 30.80 | 1.52 | 0.87     | 0.88 | 3.70  | 0.92 | 0.89     | 0.89 | 0.00  | 0.49 |
| SS                | 0.07                 | 0.44 | 99.20 | 2.81 | 0.07     | 0.32 | 99.70 | 1.84 | 0.06     | 0.22 | 97.40 | 1.06 |
| GLOBAL $-\ell_2$  | 0.31                 | 0.48 | 97.00 | 2.27 | 0.37     | 0.48 | 91.00 | 1.60 | 0.40     | 0.47 | 62.80 | 0.92 |
| GLOBAL $-\ell_1$  | 0.10                 | 0.55 | 96.10 | 2.22 | 0.13     | 0.49 | 94.40 | 1.81 | 0.09     | 0.56 | 82.90 | 1.52 |
| Specification IV  |                      |      |       |      |          |      |       |      |          |      |       |      |
| Target-Only       | 0.10                 | 0.83 | 95.30 | 3.33 | 0.12     | 0.78 | 96.10 | 3.30 | 0.12     | 0.84 | 95.90 | 3.38 |
| SS (naive)        | 0.81                 | 0.83 | 38.80 | 1.63 | 0.85     | 0.86 | 5.60  | 0.96 | 0.86     | 0.87 | 0.20  | 0.51 |
| SS                | 0.05                 | 0.44 | 99.70 | 2.89 | 0.04     | 0.32 | 99.90 | 1.87 | 0.03     | 0.21 | 98.30 | 1.06 |
| GLOBAL $-\ell_2$  | 0.29                 | 0.48 | 97.70 | 2.42 | 0.36     | 0.48 | 92.30 | 1.68 | 0.39     | 0.46 | 64.50 | 0.96 |
| GLOBAL $-\ell_1$  | 0.07                 | 0.56 | 95.70 | 2.31 | 0.09     | 0.50 | 93.60 | 1.85 | 0.06     | 0.58 | 82.00 | 1.54 |
| Specification V   |                      |      |       |      |          |      |       |      |          |      |       |      |
| Target-Only       | 0.01                 | 0.82 | 95.90 | 3.32 | 0.01     | 0.74 | 97.40 | 3.31 | 0.00     | 0.79 | 97.10 | 3.33 |
| SS (naive)        | 0.84                 | 0.86 | 30.60 | 1.53 | 0.87     | 0.88 | 3.40  | 0.90 | 0.89     | 0.89 | 0.00  | 0.49 |
| SS                | 0.08                 | 0.44 | 99.50 | 2.88 | 0.06     | 0.32 | 99.60 | 1.85 | 0.06     | 0.22 | 97.70 | 1.05 |
| GLOBAL $-\ell_2$  | 0.34                 | 0.50 | 96.70 | 2.33 | 0.40     | 0.50 | 89.10 | 1.60 | 0.43     | 0.49 | 57.70 | 0.92 |
| GLOBAL $-\ell_1$  | 0.14                 | 0.56 | 95.40 | 2.27 | 0.16     | 0.53 | 93.10 | 1.81 | 0.14     | 0.59 | 81.10 | 1.52 |

Abbreviations: RMSE = Root mean square error; Cov. = Coverage, Len. = Length of 95% CI;  
SS = Sample Size.

Table 3: Results from 1000 simulated datasets for covariate distribution  $\mathcal{D}_{\text{dense}}$  when  $P = 2$  with varying simulation settings and numbers of source sites.

|                   | Simulation scenarios |      |       |      |          |      |       |      |          |      |       |      |
|-------------------|----------------------|------|-------|------|----------|------|-------|------|----------|------|-------|------|
|                   | $K = 10$             |      |       |      | $K = 20$ |      |       |      | $K = 50$ |      |       |      |
|                   | Bias                 | RMSE | Cov.  | Len. | Bias     | RMSE | Cov.  | Len. | Bias     | RMSE | Cov.  | Len. |
| Specification I   |                      |      |       |      |          |      |       |      |          |      |       |      |
| Target-Only       | 0.00                 | 0.69 | 98.10 | 3.10 | 0.00     | 0.69 | 98.20 | 3.10 | 0.00     | 0.69 | 98.20 | 3.10 |
| SS (naive)        | 0.35                 | 0.39 | 91.50 | 1.31 | 0.28     | 0.31 | 75.60 | 0.77 | 0.27     | 0.28 | 22.80 | 0.42 |
| SS                | 0.00                 | 0.44 | 99.80 | 2.60 | 0.00     | 0.31 | 98.90 | 1.53 | 0.01     | 0.21 | 95.50 | 0.88 |
| GLOBAL $-\ell_2$  | 0.08                 | 0.26 | 98.60 | 1.43 | 0.06     | 0.20 | 95.10 | 0.86 | 0.07     | 0.17 | 87.30 | 0.50 |
| GLOBAL $-\ell_1$  | 0.04                 | 0.39 | 98.00 | 1.63 | 0.03     | 0.31 | 96.20 | 1.18 | 0.03     | 0.26 | 91.70 | 0.88 |
| Specification II  |                      |      |       |      |          |      |       |      |          |      |       |      |
| Target-Only       | 0.00                 | 0.72 | 97.50 | 3.18 | 0.00     | 0.72 | 97.60 | 3.18 | 0.00     | 0.72 | 97.60 | 3.18 |
| SS (naive)        | 0.35                 | 0.39 | 92.00 | 1.35 | 0.28     | 0.31 | 77.60 | 0.79 | 0.27     | 0.28 | 24.90 | 0.43 |
| SS                | 0.00                 | 0.45 | 99.80 | 2.65 | 0.00     | 0.31 | 98.80 | 1.56 | 0.01     | 0.21 | 95.40 | 0.90 |
| GLOBAL $-\ell_2$  | 0.08                 | 0.27 | 98.60 | 1.48 | 0.07     | 0.21 | 95.30 | 0.89 | 0.07     | 0.16 | 88.50 | 0.52 |
| GLOBAL $-\ell_1$  | 0.04                 | 0.40 | 97.90 | 1.67 | 0.04     | 0.31 | 96.40 | 1.19 | 0.04     | 0.26 | 92.60 | 0.88 |
| Specification III |                      |      |       |      |          |      |       |      |          |      |       |      |
| Target-Only       | 0.04                 | 0.71 | 96.50 | 3.09 | 0.04     | 0.70 | 96.60 | 3.09 | 0.04     | 0.70 | 96.60 | 3.09 |
| SS (naive)        | 0.32                 | 0.35 | 94.80 | 1.34 | 0.25     | 0.27 | 85.00 | 0.79 | 0.23     | 0.24 | 40.00 | 0.43 |
| SS                | 0.03                 | 0.45 | 99.80 | 2.68 | 0.03     | 0.31 | 99.10 | 1.57 | 0.03     | 0.21 | 96.10 | 0.90 |
| GLOBAL $-\ell_2$  | 0.04                 | 0.25 | 99.10 | 1.44 | 0.02     | 0.20 | 95.80 | 0.87 | 0.02     | 0.15 | 90.00 | 0.51 |
| GLOBAL $-\ell_1$  | 0.00                 | 0.40 | 96.90 | 1.63 | 0.01     | 0.31 | 95.00 | 1.18 | 0.01     | 0.26 | 91.00 | 0.87 |
| Specification IV  |                      |      |       |      |          |      |       |      |          |      |       |      |
| Target-Only       | 0.10                 | 0.74 | 96.80 | 3.18 | 0.10     | 0.74 | 96.80 | 3.18 | 0.10     | 0.74 | 96.80 | 3.18 |
| SS (naive)        | 0.28                 | 0.33 | 97.30 | 1.41 | 0.21     | 0.24 | 91.70 | 0.82 | 0.19     | 0.21 | 61.00 | 0.44 |
| SS                | 0.06                 | 0.46 | 99.80 | 2.73 | 0.06     | 0.32 | 99.20 | 1.60 | 0.06     | 0.22 | 95.90 | 0.92 |
| GLOBAL $-\ell_2$  | 0.01                 | 0.26 | 99.30 | 1.50 | 0.02     | 0.20 | 96.70 | 0.90 | 0.02     | 0.15 | 90.40 | 0.52 |
| GLOBAL $-\ell_1$  | 0.04                 | 0.41 | 97.10 | 1.67 | 0.05     | 0.31 | 94.50 | 1.18 | 0.05     | 0.26 | 88.50 | 0.86 |
| Specification V   |                      |      |       |      |          |      |       |      |          |      |       |      |
| Target-Only       | 0.00                 | 0.72 | 97.50 | 3.18 | 0.00     | 0.72 | 97.60 | 3.18 | 0.00     | 0.72 | 97.60 | 3.18 |
| SS (naive)        | 0.33                 | 0.37 | 93.90 | 1.35 | 0.27     | 0.29 | 81.90 | 0.79 | 0.25     | 0.26 | 32.60 | 0.43 |
| SS                | 0.01                 | 0.45 | 99.80 | 2.71 | 0.00     | 0.31 | 98.80 | 1.59 | 0.00     | 0.21 | 95.90 | 0.92 |
| GLOBAL $-\ell_2$  | 0.07                 | 0.26 | 98.70 | 1.47 | 0.06     | 0.20 | 95.80 | 0.89 | 0.06     | 0.16 | 89.60 | 0.52 |
| GLOBAL $-\ell_1$  | 0.04                 | 0.39 | 98.20 | 1.65 | 0.03     | 0.31 | 96.30 | 1.18 | 0.03     | 0.25 | 92.80 | 0.87 |

Abbreviations: RMSE = Root mean square error; Cov. = Coverage, Len. = Length of 95% CI;  
SS = Sample Size.

Table 4: Results from 1000 simulated datasets for covariate distribution  $\mathcal{D}_{\text{dense}}$  when  $P = 10$  with varying simulation settings and numbers of source sites.

|                   | Simulation scenarios |      |        |      |          |      |        |      |          |      |       |      |
|-------------------|----------------------|------|--------|------|----------|------|--------|------|----------|------|-------|------|
|                   | $K = 10$             |      |        |      | $K = 20$ |      |        |      | $K = 50$ |      |       |      |
|                   | Bias                 | RMSE | Cov.   | Len. | Bias     | RMSE | Cov.   | Len. | Bias     | RMSE | Cov.  | Len. |
| Specification I   |                      |      |        |      |          |      |        |      |          |      |       |      |
| Target-Only       | 0.13                 | 2.63 | 95.30  | 7.46 | 0.13     | 2.63 | 95.30  | 7.46 | 0.13     | 2.63 | 95.30 | 7.46 |
| SS (naive)        | 0.22                 | 0.46 | 99.50  | 5.09 | 0.19     | 0.33 | 99.00  | 2.89 | 0.18     | 0.25 | 94.90 | 1.40 |
| SS                | 0.00                 | 0.70 | 100.00 | 7.65 | 0.01     | 0.47 | 99.80  | 4.27 | 0.01     | 0.31 | 99.70 | 2.19 |
| GLOBAL $-\ell_2$  | 0.06                 | 0.53 | 99.80  | 6.31 | 0.07     | 0.38 | 99.40  | 3.45 | 0.07     | 0.25 | 98.40 | 1.71 |
| GLOBAL $-\ell_1$  | 0.01                 | 0.80 | 98.40  | 5.76 | 0.04     | 0.57 | 97.60  | 3.42 | 0.06     | 0.40 | 95.90 | 1.83 |
| Specification II  |                      |      |        |      |          |      |        |      |          |      |       |      |
| Target-Only       | 0.10                 | 2.50 | 95.40  | 7.55 | 0.10     | 2.50 | 95.40  | 7.55 | 0.10     | 2.50 | 95.40 | 7.55 |
| SS (naive)        | 0.22                 | 0.46 | 99.40  | 4.89 | 0.19     | 0.34 | 99.20  | 2.78 | 0.18     | 0.25 | 95.70 | 1.36 |
| SS                | 0.00                 | 0.72 | 100.00 | 7.52 | 0.01     | 0.48 | 99.80  | 4.19 | 0.01     | 0.31 | 99.60 | 2.17 |
| GLOBAL $-\ell_2$  | 0.07                 | 0.54 | 99.90  | 6.14 | 0.08     | 0.38 | 99.40  | 3.36 | 0.08     | 0.25 | 98.60 | 1.69 |
| GLOBAL $-\ell_1$  | 0.04                 | 0.82 | 98.10  | 5.53 | 0.06     | 0.57 | 97.40  | 3.30 | 0.07     | 0.41 | 96.50 | 1.79 |
| Specification III |                      |      |        |      |          |      |        |      |          |      |       |      |
| Target-Only       | 0.12                 | 2.06 | 93.20  | 7.08 | 0.12     | 2.06 | 93.20  | 7.08 | 0.12     | 2.06 | 93.20 | 7.08 |
| SS (naive)        | 0.19                 | 0.46 | 99.70  | 4.12 | 0.17     | 0.33 | 99.00  | 2.41 | 0.16     | 0.25 | 95.30 | 1.23 |
| SS                | 0.03                 | 0.87 | 100.00 | 8.11 | 0.01     | 0.59 | 100.00 | 4.63 | 0.02     | 0.38 | 99.90 | 2.42 |
| GLOBAL $-\ell_2$  | 0.02                 | 0.53 | 99.40  | 5.23 | 0.04     | 0.37 | 99.60  | 2.92 | 0.04     | 0.24 | 98.80 | 1.51 |
| GLOBAL $-\ell_1$  | 0.01                 | 0.84 | 97.70  | 4.52 | 0.01     | 0.60 | 97.50  | 2.82 | 0.03     | 0.38 | 96.30 | 1.57 |
| Specification IV  |                      |      |        |      |          |      |        |      |          |      |       |      |
| Target-Only       | 0.21                 | 2.01 | 92.90  | 7.16 | 0.21     | 2.01 | 92.90  | 7.16 | 0.21     | 2.01 | 92.90 | 7.16 |
| SS (naive)        | 0.08                 | 0.44 | 99.70  | 4.09 | 0.06     | 0.30 | 99.70  | 2.40 | 0.06     | 0.20 | 98.40 | 1.23 |
| SS                | 0.14                 | 0.89 | 100.00 | 8.12 | 0.13     | 0.62 | 99.90  | 4.70 | 0.12     | 0.41 | 99.70 | 2.44 |
| GLOBAL $-\ell_2$  | 0.09                 | 0.55 | 99.30  | 5.25 | 0.07     | 0.38 | 99.20  | 2.92 | 0.06     | 0.25 | 99.10 | 1.51 |
| GLOBAL $-\ell_1$  | 0.11                 | 0.86 | 97.40  | 4.44 | 0.10     | 0.62 | 96.60  | 2.80 | 0.07     | 0.41 | 95.10 | 1.57 |
| Specification V   |                      |      |        |      |          |      |        |      |          |      |       |      |
| Target-Only       | 0.10                 | 2.50 | 95.40  | 7.55 | 0.10     | 2.50 | 95.40  | 7.55 | 0.10     | 2.50 | 95.40 | 7.55 |
| SS (naive)        | 0.15                 | 0.45 | 99.80  | 4.97 | 0.13     | 0.32 | 99.30  | 2.84 | 0.12     | 0.22 | 97.70 | 1.40 |
| SS                | 0.07                 | 0.89 | 100.00 | 9.00 | 0.05     | 0.61 | 99.90  | 5.14 | 0.05     | 0.39 | 99.80 | 2.60 |
| GLOBAL $-\ell_2$  | 0.01                 | 0.55 | 99.80  | 6.14 | 0.03     | 0.37 | 99.60  | 3.36 | 0.02     | 0.24 | 98.40 | 1.69 |
| GLOBAL $-\ell_1$  | 0.00                 | 0.82 | 98.50  | 5.52 | 0.00     | 0.57 | 97.70  | 3.31 | 0.03     | 0.41 | 96.10 | 1.81 |

Abbreviations: RMSE = Root mean square error; Cov. = Coverage, Len. = Length of 95% CI;  
SS = Sample Size.

Table 5: Results from 500 simulated datasets when  $P = 2$  anchoring total population with varying simulation settings and numbers of source sites. The true effects are uniform across all the sites in Setting  $\text{GATE}_{\text{uniform}}$  and vary in Setting  $\text{GATE}_{\text{various}}$ .

|                               | Simulation scenarios |      |       |      |          |      |       |      |          |      |       |      |
|-------------------------------|----------------------|------|-------|------|----------|------|-------|------|----------|------|-------|------|
|                               | $K = 10$             |      |       |      | $K = 20$ |      |       |      | $K = 50$ |      |       |      |
|                               | Bias                 | RMSE | Cov.  | Len. | Bias     | RMSE | Cov.  | Len. | Bias     | RMSE | Cov.  | Len. |
| <b>GATE<sub>uniform</sub></b> |                      |      |       |      |          |      |       |      |          |      |       |      |
| Specification I               |                      |      |       |      |          |      |       |      |          |      |       |      |
| Target-Only                   | 0.02                 | 0.69 | 98.00 | 3.11 | 0.02     | 0.69 | 98.00 | 3.12 | 0.02     | 0.69 | 98.00 | 3.12 |
| SS (naive)                    | 0.00                 | 0.15 | 99.00 | 0.98 | 0.00     | 0.11 | 99.00 | 0.62 | 0.01     | 0.07 | 98.80 | 0.36 |
| SS                            | 0.00                 | 0.16 | 99.20 | 0.97 | 0.00     | 0.11 | 98.80 | 0.62 | 0.01     | 0.07 | 98.80 | 0.36 |
| GLOBAL $-\ell_2$              | 0.04                 | 0.18 | 99.40 | 1.07 | 0.04     | 0.14 | 98.60 | 0.69 | 0.04     | 0.09 | 97.60 | 0.40 |
| GLOBAL $-\ell_1$              | 0.03                 | 0.27 | 99.20 | 1.29 | 0.03     | 0.22 | 99.40 | 0.97 | 0.03     | 0.17 | 98.60 | 0.73 |
| Fixed-effects                 | 0.02                 | 0.63 | 95.20 | 2.42 | 0.01     | 0.63 | 95.00 | 2.42 | 0.01     | 0.63 | 94.60 | 2.41 |
| Specification II              |                      |      |       |      |          |      |       |      |          |      |       |      |
| Target-Only                   | 0.04                 | 0.83 | 95.40 | 3.43 | 0.04     | 0.84 | 95.40 | 3.44 | 0.04     | 0.84 | 95.40 | 3.44 |
| SS (naive)                    | 0.00                 | 0.18 | 99.00 | 1.18 | 0.01     | 0.13 | 99.00 | 0.74 | 0.01     | 0.08 | 98.60 | 0.42 |
| SS                            | 0.01                 | 0.18 | 99.00 | 1.19 | 0.01     | 0.13 | 98.80 | 0.75 | 0.02     | 0.08 | 98.20 | 0.42 |
| GLOBAL $-\ell_2$              | 0.00                 | 0.20 | 99.00 | 1.26 | 0.01     | 0.15 | 99.00 | 0.80 | 0.01     | 0.09 | 97.60 | 0.46 |
| GLOBAL $-\ell_1$              | 0.01                 | 0.28 | 98.60 | 1.41 | 0.02     | 0.22 | 97.80 | 1.01 | 0.02     | 0.17 | 96.40 | 0.70 |
| Fixed-effects                 | 0.14                 | 0.69 | 95.20 | 2.64 | 0.14     | 0.69 | 95.40 | 2.63 | 0.13     | 0.69 | 95.80 | 2.63 |
| <b>GATE<sub>various</sub></b> |                      |      |       |      |          |      |       |      |          |      |       |      |
| Specification I               |                      |      |       |      |          |      |       |      |          |      |       |      |
| Target-Only                   | 0.02                 | 0.69 | 98.00 | 3.11 | 0.02     | 0.69 | 98.00 | 3.12 | 0.02     | 0.69 | 98.00 | 3.12 |
| SS (naive)                    | 0.32                 | 0.42 | 93.20 | 1.38 | 0.28     | 0.35 | 76.00 | 0.82 | 0.25     | 0.28 | 40.20 | 0.44 |
| SS                            | 0.32                 | 0.42 | 93.00 | 1.38 | 0.28     | 0.35 | 75.60 | 0.83 | 0.25     | 0.28 | 40.40 | 0.44 |
| GLOBAL $-\ell_2$              | 0.12                 | 0.25 | 97.40 | 1.20 | 0.07     | 0.18 | 94.60 | 0.75 | 0.03     | 0.12 | 92.20 | 0.42 |
| GLOBAL $-\ell_1$              | 0.09                 | 0.31 | 99.20 | 1.40 | 0.05     | 0.26 | 98.00 | 1.07 | 0.02     | 0.21 | 95.80 | 0.81 |
| Fixed-effects                 | 0.02                 | 0.63 | 95.20 | 2.42 | 0.01     | 0.63 | 95.00 | 2.42 | 0.01     | 0.63 | 94.60 | 2.41 |
| Specification II              |                      |      |       |      |          |      |       |      |          |      |       |      |
| Target-Only                   | 0.04                 | 0.83 | 95.40 | 3.43 | 0.04     | 0.84 | 95.40 | 3.44 | 0.04     | 0.84 | 95.40 | 3.44 |
| SS (naive)                    | 0.32                 | 0.43 | 94.80 | 1.60 | 0.28     | 0.35 | 83.00 | 0.95 | 0.24     | 0.28 | 52.80 | 0.50 |
| SS                            | 0.31                 | 0.43 | 95.20 | 1.61 | 0.28     | 0.35 | 83.60 | 0.95 | 0.24     | 0.27 | 56.00 | 0.50 |
| GLOBAL $-\ell_2$              | 0.06                 | 0.24 | 98.60 | 1.39 | 0.00     | 0.18 | 96.40 | 0.86 | 0.04     | 0.13 | 91.80 | 0.48 |
| GLOBAL $-\ell_1$              | 0.03                 | 0.32 | 98.60 | 1.52 | 0.01     | 0.27 | 96.40 | 1.09 | 0.05     | 0.21 | 93.20 | 0.77 |
| Fixed-effects                 | 0.14                 | 0.69 | 95.20 | 2.64 | 0.14     | 0.69 | 95.40 | 2.63 | 0.13     | 0.69 | 95.80 | 2.63 |

Abbreviations: RMSE = Root mean square error; Cov. = Coverage, Len. = Length of 95% CI.

Table 6: Results from 500 simulated datasets when  $P = 10$  anchoring total population with varying simulation settings and numbers of source sites. The true effects are uniform across all the sites.

|                               | Simulation scenarios |      |       |      |          |      |       |      |          |      |       |      |
|-------------------------------|----------------------|------|-------|------|----------|------|-------|------|----------|------|-------|------|
|                               | $K = 10$             |      |       |      | $K = 20$ |      |       |      | $K = 50$ |      |       |      |
|                               | Bias                 | RMSE | Cov.  | Len. | Bias     | RMSE | Cov.  | Len. | Bias     | RMSE | Cov.  | Len. |
| <b>GATE<sub>uniform</sub></b> |                      |      |       |      |          |      |       |      |          |      |       |      |
| Specification I               |                      |      |       |      |          |      |       |      |          |      |       |      |
| Target-Only                   | 0.11                 | 3.48 | 95.60 | 8.42 | 0.11     | 3.41 | 95.80 | 8.41 | 0.09     | 3.26 | 95.80 | 8.37 |
| SS (naive)                    | 0.04                 | 0.42 | 99.80 | 6.37 | 0.01     | 0.28 | 99.40 | 3.57 | 0.01     | 0.18 | 99.60 | 1.68 |
| SS                            | 0.04                 | 0.43 | 99.60 | 7.16 | 0.02     | 0.28 | 99.20 | 3.90 | 0.01     | 0.18 | 99.40 | 1.73 |
| global $-\ell_2$              | 0.02                 | 0.48 | 99.80 | 7.22 | 0.04     | 0.33 | 99.60 | 3.92 | 0.04     | 0.21 | 98.80 | 1.75 |
| global $-\ell_1$              | 0.03                 | 0.58 | 99.40 | 7.24 | 0.05     | 0.43 | 97.40 | 4.06 | 0.05     | 0.30 | 96.20 | 2.01 |
| Fixed-effects                 | 0.05                 | 1.36 | 93.20 | 5.33 | 0.03     | 1.36 | 94.00 | 5.31 | 0.03     | 1.36 | 93.60 | 5.30 |
| Specification II              |                      |      |       |      |          |      |       |      |          |      |       |      |
| Target-Only                   | 0.10                 | 3.14 | 93.80 | 8.96 | 0.10     | 3.10 | 93.60 | 8.97 | 0.09     | 3.04 | 94.20 | 8.95 |
| SS (naive)                    | 0.05                 | 0.44 | 99.60 | 6.11 | 0.03     | 0.31 | 99.80 | 3.46 | 0.03     | 0.20 | 98.60 | 1.67 |
| SS                            | 0.08                 | 0.46 | 99.80 | 6.55 | 0.07     | 0.32 | 99.40 | 3.63 | 0.06     | 0.21 | 98.80 | 1.72 |
| global $-\ell_2$              | 0.10                 | 0.51 | 99.80 | 6.59 | 0.09     | 0.37 | 99.00 | 3.64 | 0.09     | 0.24 | 97.60 | 1.72 |
| global $-\ell_1$              | 0.12                 | 0.72 | 98.60 | 6.41 | 0.09     | 0.48 | 98.00 | 3.63 | 0.09     | 0.34 | 96.00 | 1.78 |
| Fixed-effects                 | 0.28                 | 1.50 | 93.80 | 5.87 | 0.26     | 1.50 | 93.40 | 5.84 | 0.26     | 1.50 | 94.00 | 5.83 |
| <b>GATE<sub>various</sub></b> |                      |      |       |      |          |      |       |      |          |      |       |      |
| Specification I               |                      |      |       |      |          |      |       |      |          |      |       |      |
| Target-Only                   | 0.11                 | 3.48 | 95.60 | 8.42 | 0.11     | 3.41 | 95.80 | 8.41 | 0.09     | 3.26 | 95.80 | 8.37 |
| Target-Only                   | 0.29                 | 0.57 | 98.80 | 6.79 | 0.28     | 0.42 | 97.40 | 3.82 | 0.25     | 0.32 | 90.60 | 1.76 |
| SS                            | 0.29                 | 0.58 | 99.40 | 7.58 | 0.27     | 0.43 | 97.80 | 4.14 | 0.25     | 0.32 | 92.20 | 1.81 |
| global $-\ell_2$              | 0.06                 | 0.51 | 99.40 | 7.32 | 0.03     | 0.35 | 99.40 | 3.97 | 0.01     | 0.23 | 97.60 | 1.77 |
| global $-\ell_1$              | 0.08                 | 0.64 | 98.80 | 7.38 | 0.03     | 0.49 | 97.80 | 4.04 | 0.00     | 0.32 | 96.60 | 2.00 |
| Fixed-effects                 | 0.05                 | 1.36 | 93.20 | 5.33 | 0.03     | 1.36 | 94.00 | 5.31 | 0.03     | 1.36 | 93.60 | 5.30 |
| Specification II              |                      |      |       |      |          |      |       |      |          |      |       |      |
| Target-Only                   | 0.10                 | 3.14 | 93.80 | 8.96 | 0.10     | 3.10 | 93.60 | 8.97 | 0.09     | 3.04 | 94.20 | 8.95 |
| SS (naive)                    | 0.27                 | 0.57 | 99.40 | 6.55 | 0.25     | 0.44 | 98.60 | 3.67 | 0.22     | 0.32 | 93.60 | 1.74 |
| SS                            | 0.24                 | 0.57 | 99.80 | 7.01 | 0.22     | 0.42 | 99.00 | 3.84 | 0.19     | 0.29 | 96.80 | 1.79 |
| global $-\ell_2$              | 0.06                 | 0.52 | 99.80 | 6.69 | 0.11     | 0.39 | 99.40 | 3.68 | 0.14     | 0.29 | 95.60 | 1.74 |
| global $-\ell_1$              | 0.09                 | 0.73 | 98.20 | 6.48 | 0.12     | 0.52 | 98.00 | 3.67 | 0.13     | 0.37 | 94.20 | 1.79 |
| Fixed-effects                 | 0.28                 | 1.50 | 93.80 | 5.87 | 0.26     | 1.50 | 93.40 | 5.84 | 0.26     | 1.50 | 94.00 | 5.83 |

Abbreviations: RMSE = Root mean square error; Cov. = Coverage, Len. = Length of 95% CI.

## Weights for the dense covariate setting

Recall that in the main text, we displayed the  $\eta_k$  weights for  $k = 1, \dots, K$  when  $K = 20$  hospitals in the sparse setting. Here, we illustrate the  $\eta_k$  weights, again for  $K = 20$  hospitals, but for the dense setting. Figure 3 summarizes the results. The global  $-\ell_1$  estimator places about 40% of the weight on the target hospital and drops some sites entirely that have large bias compared to the target site TATE. The SS estimator has the same weights as in the  $\mathcal{D}_{\text{sparse}}$  setting. As in the  $\mathcal{D}_{\text{sparse}}$  setting, the global  $-\ell_2$  estimator produces weights between

the global  $-\ell_1$  estimator and the SS estimator. In terms of covariate imbalance, there is less difference between the global  $-\ell_1$  and global  $-\ell_2$  estimators, so the global  $-\ell_2$  estimator may be preferable as it has a larger effective sample size and thus smaller variance since it drops fewer sites. In the  $\mathcal{D}_{\text{dense}}$  setting, the differences in covariate imbalances using the global  $-\ell_1$ , global  $-\ell_2$ , and SS estimators are less pronounced. In this setting, the global  $-\ell_2$  estimator is preferred to the global  $-\ell_1$  estimator due to its smaller RMSE.

# Appendix IV. Additional Real Data Analysis Results

## Covariate Balance Diagnostics

In addition to 30-day mortality, we also study the causal effect of PCI versus MM on patient length of stay. Detailed covariate balance diagnostics for indirect standardization and direct standardization are provided in the tables below.

Table 7: Covariate balance diagnostics for LOS as the outcome (indirect standardization)

| Hospital A       | Goal Hosp A | PCI Hosp A | MM Source | PCI Source | MM Tgt-Only | PCI Tgt-Only | MM Global- $\ell_1$ | PCI Global- $\ell_1$ | MM    |
|------------------|-------------|------------|-----------|------------|-------------|--------------|---------------------|----------------------|-------|
| Covariates       |             |            |           |            |             |              |                     |                      |       |
| Age              | 80.52       | 79.11      | 81.67     | 76.52      | 79.24       | 80.52        | 80.52               | 80.52                | 80.52 |
| Female           | 0.45        | 0.38       | 0.51      | 0.41       | 0.46        | 0.45         | 0.45                | 0.45                 | 0.45  |
| History of PCI   | 0.23        | 0.28       | 0.19      | 0.23       | 0.22        | 0.23         | 0.23                | 0.23                 | 0.23  |
| Renal Disease    | 0.45        | 0.43       | 0.47      | 0.29       | 0.45        | 0.45         | 0.45                | 0.45                 | 0.45  |
| Eff. sample size |             | 81         | 100       | 4923       | 5999        | 68           | 51                  | 1321                 | 1818  |
| Hospital B       | Goal Hosp A | PCI Hosp A | MM Source | PCI Source | MM Tgt-Only | PCI Tgt-Only | MM Global- $\ell_1$ | PCI Global- $\ell_1$ | MM    |
| Covariates       |             |            |           |            |             |              |                     |                      |       |
| Age              | 75.89       | 75.56      | 76.12     | 76.58      | 79.34       | 75.89        | 75.89               | 75.89                | 75.89 |
| Female           | 0.36        | 0.33       | 0.38      | 0.41       | 0.46        | 0.36         | 0.36                | 0.36                 | 0.36  |
| History of PCI   | 0.18        | 0.18       | 0.18      | 0.24       | 0.22        | 0.18         | 0.18                | 0.18                 | 0.18  |
| Renal Disease    | 0.32        | 0.29       | 0.34      | 0.30       | 0.45        | 0.32         | 0.32                | 0.32                 | 0.32  |
| Eff. sample size |             | 91         | 128       | 4913       | 5971        | 76           | 110                 | 1475                 | 1349  |
| Hospital C       | Goal Hosp A | PCI Hosp A | MM Source | PCI Source | MM Tgt-Only | PCI Tgt-Only | MM Global- $\ell_1$ | PCI Global- $\ell_1$ | MM    |
| Covariates       |             |            |           |            |             |              |                     |                      |       |
| Age              | 78.70       | 77.02      | 80.35     | 76.56      | 79.26       | 78.70        | 78.70               | 78.70                | 78.70 |
| Female           | 0.49        | 0.49       | 0.48      | 0.40       | 0.46        | 0.49         | 0.49                | 0.49                 | 0.49  |
| History of PCI   | 0.25        | 0.25       | 0.24      | 0.23       | 0.21        | 0.25         | 0.25                | 0.25                 | 0.25  |
| Renal Disease    | 0.40        | 0.30       | 0.50      | 0.29       | 0.45        | 0.40         | 0.40                | 0.40                 | 0.40  |
| Eff. sample size |             | 87         | 88        | 4917       | 6011        | 72           | 60                  | 1357                 | 1415  |

Table 8: Covariate balance diagnostics for LOS as the outcome (direct standardization)

| Hospital A       | Goal Hosp A | PCI Hosp A | MM Source | PCI Source | MM Tgt-Only | PCI Tgt-Only | MM Global- $\ell_1$ | PCI Global- $\ell_1$ | MM    |
|------------------|-------------|------------|-----------|------------|-------------|--------------|---------------------|----------------------|-------|
| Covariates       |             |            |           |            |             |              |                     |                      |       |
| Age              | 78.05       | 79.11      | 81.67     | 76.52      | 79.24       | 78.05        | 78.05               | 78.05                | 78.05 |
| Female           | 0.44        | 0.38       | 0.51      | 0.41       | 0.46        | 0.44         | 0.44                | 0.44                 | 0.44  |
| History of PCI   | 0.22        | 0.28       | 0.19      | 0.23       | 0.22        | 0.22         | 0.22                | 0.22                 | 0.22  |
| Renal Disease    | 0.38        | 0.43       | 0.47      | 0.29       | 0.45        | 0.38         | 0.38                | 0.38                 | 0.38  |
| Eff. sample size |             | 81         | 100       | 4923       | 5999        | 69           | 45                  | 1660                 | 1609  |
| Hospital B       | Goal Hosp A | PCI Hosp A | MM Source | PCI Source | MM Tgt-Only | PCI Tgt-Only | MM Global- $\ell_1$ | PCI Global- $\ell_1$ | MM    |
| Covariates       |             |            |           |            |             |              |                     |                      |       |
| Age              | 78.05       | 75.56      | 76.12     | 76.58      | 79.34       | 78.05        | 78.05               | 78.05                | 78.05 |
| Female           | 0.44        | 0.33       | 0.38      | 0.41       | 0.46        | 0.44         | 0.44                | 0.44                 | 0.44  |
| History of PCI   | 0.22        | 0.18       | 0.18      | 0.24       | 0.22        | 0.22         | 0.22                | 0.22                 | 0.22  |
| Renal Disease    | 0.38        | 0.29       | 0.34      | 0.30       | 0.45        | 0.38         | 0.38                | 0.38                 | 0.38  |
| Eff. sample size |             | 91         | 128       | 4913       | 5971        | 60           | 92                  | 1606                 | 1709  |
| Hospital C       | Goal Hosp A | PCI Hosp A | MM Source | PCI Source | MM Tgt-Only | PCI Tgt-Only | MM Global- $\ell_1$ | PCI Global- $\ell_1$ | MM    |
| Covariates       |             |            |           |            |             |              |                     |                      |       |
| Age              | 78.05       | 77.02      | 80.35     | 76.56      | 79.26       | 78.05        | 78.05               | 78.05                | 78.05 |
| Female           | 0.44        | 0.49       | 0.48      | 0.40       | 0.46        | 0.44         | 0.44                | 0.44                 | 0.44  |
| History of PCI   | 0.22        | 0.25       | 0.24      | 0.23       | 0.21        | 0.22         | 0.22                | 0.22                 | 0.22  |
| Renal Disease    | 0.38        | 0.30       | 0.50      | 0.29       | 0.45        | 0.38         | 0.38                | 0.38                 | 0.38  |
| Eff. sample size |             | 87         | 88        | 4917       | 6011        | 67           | 47                  | 1345                 | 1266  |



## Causal Effect of PCI versus MM on Length of Stay

We illustrate that there is again a marked difference in hospital weights  $\boldsymbol{\eta}$  using our proposed global estimators GLOBAL- $\ell_1$  and GLOBAL- $\ell_2$  compared to SS. As before, we showcase our method with the same three diverse target hospitals. GLOBAL- $\ell_1$  places more weight on hospitals with relatively small bias, while GLOBAL- $\ell_2$  is in between GLOBAL- $\ell_1$  and the SS estimator as before. Interestingly, there is not as clear of a monotonic decreasing relationship between bias and hospital weight as in the case of 30-day mortality.

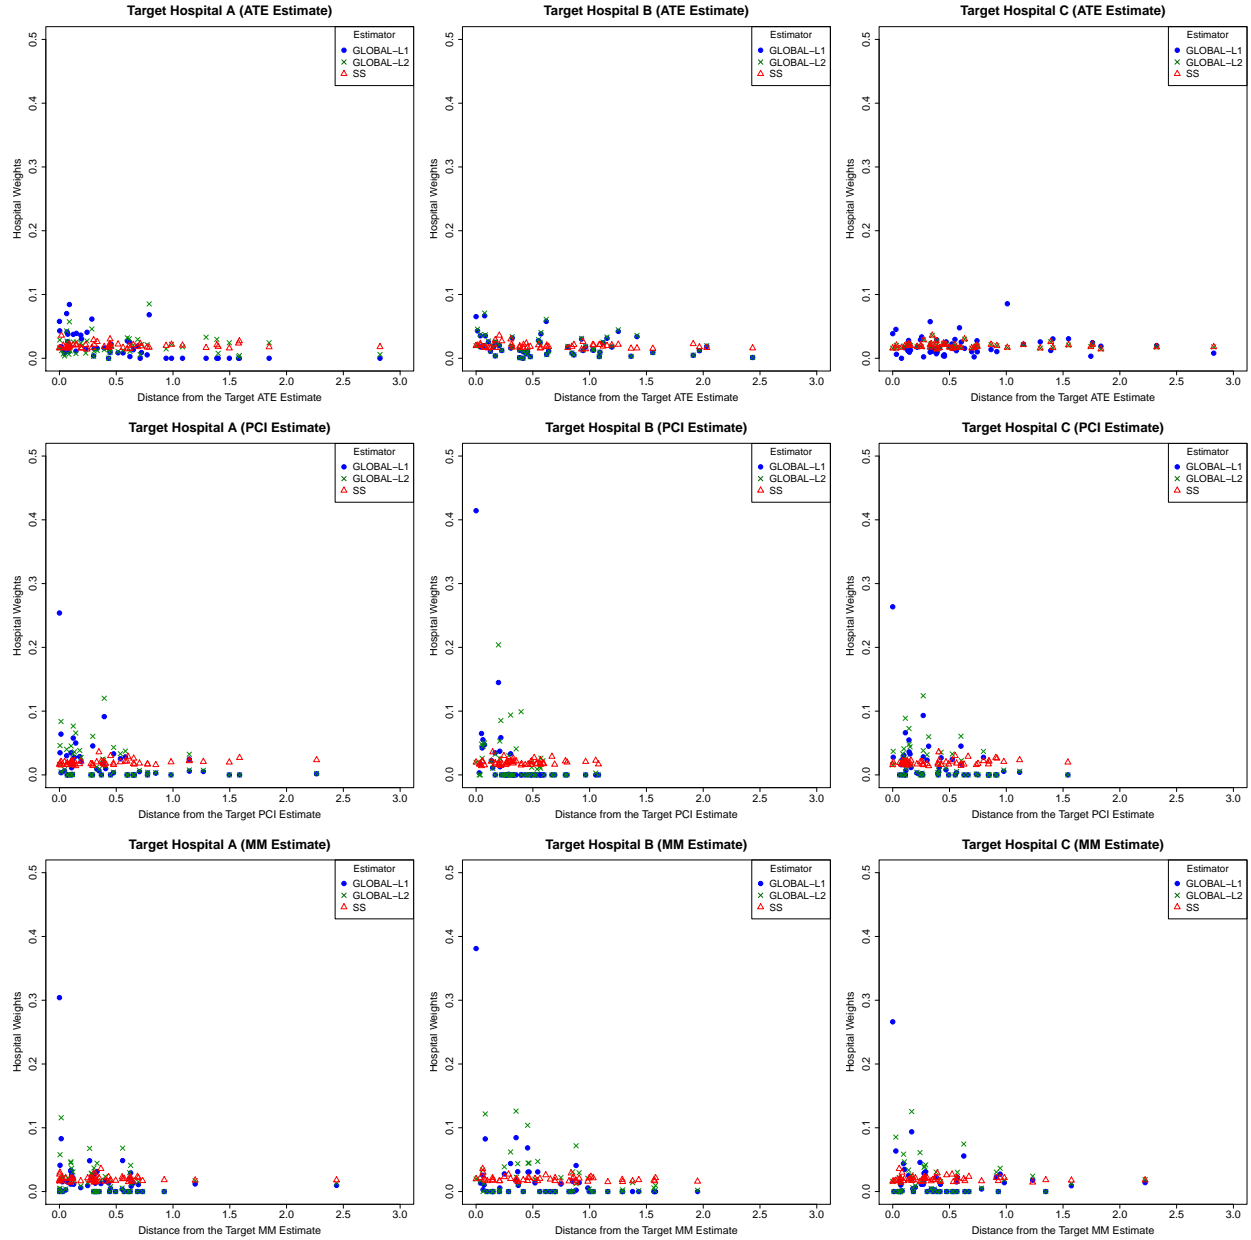

Figure 2: LOS: The global estimators place more weight on source hospitals with more similar estimates regardless of estimand, whether the target hospital is an urban major teaching hospital (A), an urban for-profit hospital (B), or a rural non-teaching hospital (C).

The causal effect of PCI versus MM on LOS was negative and statistically significant in 90% of the hospitals using our GLOBAL- $\ell_1$  estimator, compared to just 59% using the target-only estimator. The TATE is measured in days, showing that patients treated with PCI tended to have a shorter average LOS compared to MM by approximately 2 to 4 days.

Relative to the target-only estimator, the percent reduction in the 95% CI length with the GLOBAL- $\ell_1$  estimator ranged from 65% to 87% with a median of 80%. With this increased precision, 31% (16/51) of hospitals had a qualitative change in the causal effect of PCI on shorter LOS from not statistically significant to statistically significantly shorter.

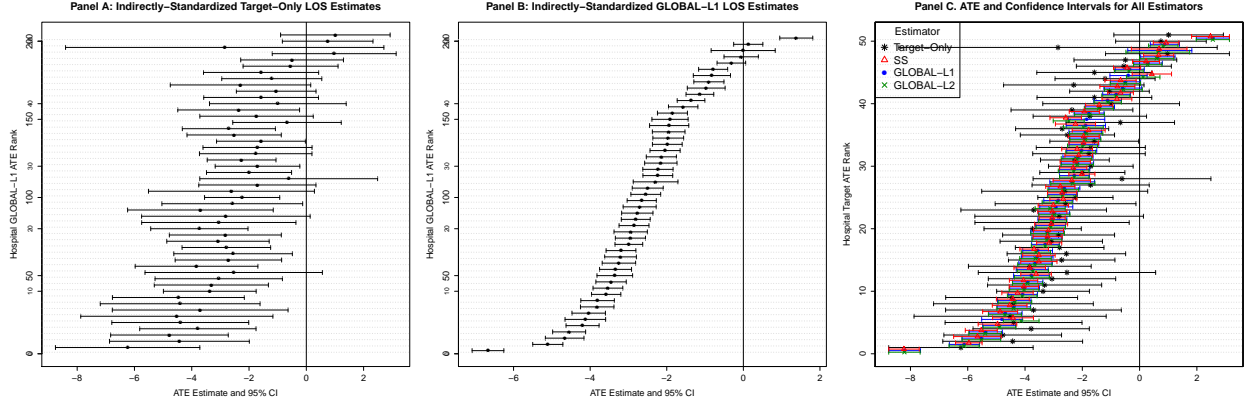

Figure 3: LOS: TATE estimates for all 51 hospitals show substantial precision gain of GLOBAL- $\ell_1$  compared to the Target-Only estimator and accuracy comparable to the GLOBAL- $\ell_2$  and SS estimators.

Figure 4 shows hospital LOS estimates for PCI and MM, with hospitals sequenced from the lowest (best) to highest (worst) PCI LOS. We find that PCI patients had shorter LOS than MM patients in all hospitals. As with 30-day mortality, very few hospitals fared particularly well on both PCI and MM rankings for LOS.

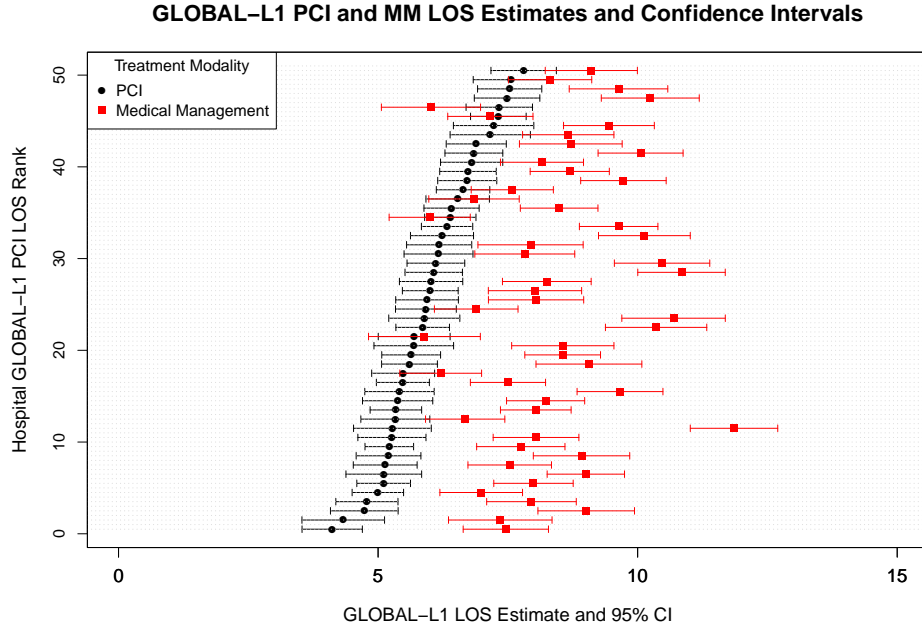

Figure 4: LOS: GLOBAL- $\ell_1$  hospital mortality estimates and 95% CIs show that hospitals that ranked highly on PCI mortality tended not to rank as well on MM and vice versa; moreover, MM mortality estimates varied considerably even among hospitals with similar PCI performance.
